# Supplementary material for: VerifiedLab: Harnessing Knowns for Unknowns
Source: arXiv:2610.37923 source file (2026-10-27)
Supplement: Supplementary file 1 [file supp_labels.tex]

\makeatletter
% Generated by scripts/sync_xrefs.py from supplementary.aux; do not edit.
\xr@def{S}{fig:database}{4}
\xr@def{S}{fig:ed-generators}{1}
\xr@def{S}{fig:ed-subfields}{2}
\xr@def{S}{fig:ed-verifiers}{3}
\xr@def{S}{fig:pred-tabular}{5}
\xr@def{S}{fig:pred-text}{6}
\xr@def{S}{fig:ws-claims}{13}
\xr@def{S}{fig:ws-data}{11}
\xr@def{S}{fig:ws-literature}{8}
\xr@def{S}{fig:ws-overview}{7}
\xr@def{S}{fig:ws-reliability}{10}
\xr@def{S}{fig:ws-session}{12}
\xr@def{S}{fig:ws-skills}{15}
\xr@def{S}{fig:ws-studio}{9}
\xr@def{S}{fig:ws-trace}{14}
\xr@def{S}{tab:scale-vs-skill}{2}
\xr@def{S}{tab:verifier-acceptance}{1}
\makeatother
